# Supplementary material for: Virtual Constraints and Hybrid Zero Dynamics for Realizing Underactuated Bipedal Locomotion
Source: arXiv:1706.01127 source file (2017-06-04)
Supplement: Supplementary file 1 [file 9-AdditionalMaterial.tex]

Here are some topics where we can write 3 or 4 sentences each, with references to the literature on HZD.

\begin{enumerate}
\item Multiple phases

\item Non-trivial double support

\item Fully actuated robots

\item Two step approach to stability

\item Composition of motions

\item Uneven ground

\item Series elastic actuators

\end{enumerate}
